# Supplementary material for: Mosaic: Efficient CPU--GPU Coordinated Block-Sparse Attention for Long-Context Decoding
Source: arXiv:2605.07719 source file (2026-11-23)
Supplement: Supplementary file 1 [file appendix.tex]

\section{Detailed Feature Definitions and Extraction}

The predictor in \sys~utilizes a total of 41 low-overhead features to capture key patterns in attention computation. We provide detailed feature definitions in Appendix~\ref{app:feature_definition}, and describe the feature extraction pipeline for both training and inference in Appendix~\ref{app:feature_extraction}.


\begin{figure}[h]
\centering
\includegraphics[width=0.92\linewidth]{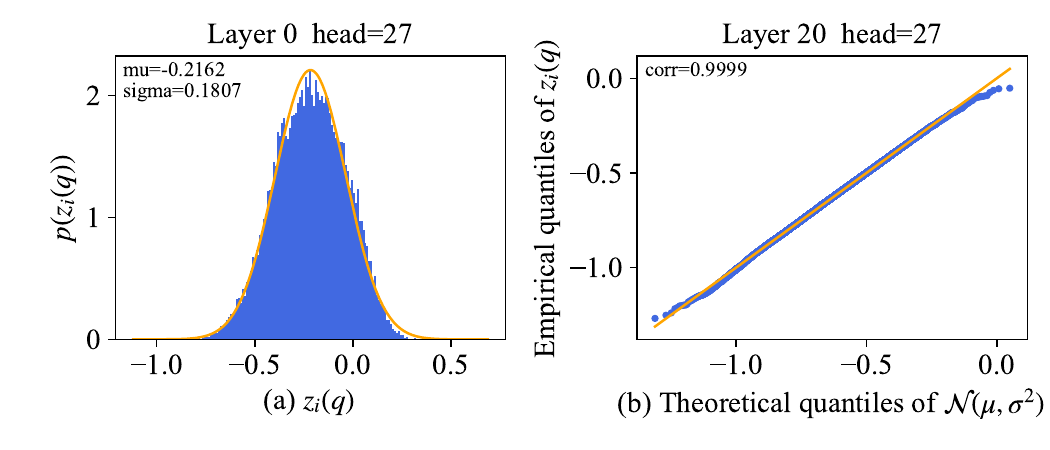}
\caption{\textbf{Normality of CPU-offloaded $q$--$k$ interactions.}
We plot $z_i(q)=\langle q,k_i\rangle/(\|q\|_2\sqrt{D})$ for CPU-offloaded keys.
(b): histogram with a fitted Gaussian density (layer 0).
(a): Q--Q plot against $\mathcal{N}(\mu,\sigma^2)$ (layer 20).
Results are from Llama-3.1-8B-Instruct on RULER with 32K context, using two representative layers.}
\Description{}
\label{fig:qk-z-normality}
\end{figure}



\subsection{Feature Definition}
\label{app:feature_definition}

We define features at a Transformer layer $\ell$ and attention head $h\in\{1,\dots,H\}$, where $H$ is the number of heads and $D$ is the per-head hidden dimension. During the prefill stage with s length $L$, the head-specific projections are
$Q\in\mathbb{R}^{L\times D},K\in\mathbb{R}^{L\times D},V\in\mathbb{R}^{L\times D}$. We partition the prefill KV cache into three disjoint segments: sink tokens ($L_{\mathrm{sink}}$), cpu tokens ($L_{\mathrm{cpu}}$), and local tokens ($L_{\mathrm{local}}$), such that $L = L_{\mathrm{sink}} + L_{\mathrm{cpu}} + L_{\mathrm{local}}$. The KV pairs corresponding to $L_{\mathrm{sink}}$ and $L_{\mathrm{local}}$ reside on GPU memory, while those corresponding to $L_{\mathrm{cpu}}$ are offloaded to host memory. Let $K_{\mathrm{sink}}\in\mathbb{R}^{L_{\mathrm{sink}}\times D}$ denote the sub-matrix of $K$ restricted to sink tokens, and similarly define
$K_{\mathrm{cpu}},K_{\mathrm{local}}$ and $V_{\mathrm{sink}},V_{\mathrm{cpu}},V_{\mathrm{local}}$.

During decoding, for each newly generated token, the model produces vectors $(q,k,v)\in\mathbb{R}^{D}$, where $q$ is the current decoding query. The newly generated KV pairs are appended to the GPU KV cache. Let $L_{\mathrm{new}}$ denote the number of generated tokens already stored in the cache when processing the current $q$. Then the GPU-resident KV length is $L_{\mathrm{gpu}} \;=\; L_{\mathrm{sink}} + L_{\mathrm{local}} + L_{\mathrm{new}}.$ We use $q'$ to denote the query of the last token in the prefill stage (the \emph{anchor query}).

We define row-wise $\ell_2$ norms over the hidden dimension $D$, denoted as $\|X\|_2$, and define the token-wise mean as averaging over the sequence (token) dimension. For a scalar vector over tokens, we define statistics along the token dimension, including mean, variance, skewness, and kurtosis. We use $\langle \cdot, \cdot \rangle$ to denote the Euclidean inner product over the hidden dimension. Then, we define the following features:

\noindent{\textbf{Structural Features (4).}}
These features describe the structural configuration of the attention module and KV cache.
\begin{itemize}
\item Layer index $\ell$.
\item Head index $h$.
\item CPU-resident KV length $L_{\mathrm{cpu}}$.
\item GPU-resident KV length $L_{\mathrm{gpu}}$.
\end{itemize}

\noindent{\textbf{KV Distribution Features (12).}}
We use $\ell_2$-type norms to characterize the distributions of $K$ and $V$ on different segments. Key norms influence attention scores directly, while value norms reflect the potential output magnitude. This distinction is especially important for sink tokens, which often receive strong attention scores but may have relatively small value magnitudes.
\begin{itemize}
\item $\|K_{\mathrm{sink}}\|_2$, $\|V_{\mathrm{sink}}\|_2$.
\item $\|\operatorname{MEAN}(K_{\mathrm{cpu}})\|_2$,
      $\|\operatorname{MEAN}(V_{\mathrm{cpu}})\|_2$.
\item $\operatorname{MEAN}(\|K_{\mathrm{cpu}}\|_{2})$,
      $\operatorname{VAR}(\|K_{\mathrm{cpu}}\|_{2})$,
      $\operatorname{SKEW}(\|K_{\mathrm{cpu}}\|_{2})$, \\
      $\operatorname{KURT}(\|K_{\mathrm{cpu}}\|_{2})$.
\item $\operatorname{MEAN}(\|V_{\mathrm{cpu}}\|_{2})$,
      $\operatorname{VAR}(\|V_{\mathrm{cpu}}\|_{2})$,
      $\operatorname{SKEW}(\|V_{\mathrm{cpu}}\|_{2})$, \\
      $\operatorname{KURT}(\|V_{\mathrm{cpu}}\|_{2})$.
\end{itemize}

\noindent{\textbf{QK Interaction Features (5).}}
For CPU-offloaded tokens, we consider the normalized inner products
\[
z_i(q) \;=\; \frac{\langle q, k_i\rangle}{\|q\|_2\,\sqrt{D}},
\qquad i\in\{1,\dots,L_{\mathrm{cpu}}\},
\]
where $k_i$ is the $i$-th row of $K_{\mathrm{cpu}}$.
Empirically, $\{z_i(q)\}_{i=1}^{L_{\mathrm{cpu}}}$ approximately follows a normal distribution across multiple models
(e.g., Llama-3.1-8B-Instruct and Qwen2.5-7B-Instruct, as shown in Fig.~\ref{fig:qk-z-normality}).
We therefore characterize this distribution via moment statistics:
\begin{itemize}
\item $\dfrac{\langle q,\operatorname{MEAN}(K_{\mathrm{cpu}})\rangle}{\|q\|_2\,\sqrt{D}}$.
\item $\operatorname{MEAN}(z(q'))$,
      $\operatorname{VAR}(z(q'))$,
      $\operatorname{SKEW}(z(q'))$, \\
      $\operatorname{KURT}(z(q'))$.
\end{itemize}
where $z(q')\in\mathbb{R}^{L_{\mathrm{cpu}}}$ is the vector whose $i$-th entry is $z_i(q')$.

\noindent{\textbf{Attention Contribution Features (11).}}
For any segment $S\in\{\mathrm{sink},\mathrm{cpu},\mathrm{local}\}$, define the score vector $s_S(q) = \frac{qK_S^\top}{\sqrt{D}}\in\mathbb{R}^{L_S}$, and the segment-wise log-sum-exp $\operatorname{LSE}(s) = \log \sum_{i} e^{s_i}$.
The segment-wise output are $O_S(q) = \operatorname{softmax}(s_S(q)) V_S \in \mathbb{R}^D$.
Intuitively, $\operatorname{LSE}(s_S(q))$ measures the unnormalized attention mass on segment $S$, while $\|O_S(q)\|_2$ captures the value-weighted output magnitude within the segment. Together, they describe the relative importance of sink/CPU/local tokens. We use the following 11 features:
\begin{itemize}
\item $\operatorname{LSE}(s_{\mathrm{sink}}(q))$,
      $\operatorname{LSE}(s_{\mathrm{cpu}}(q))$,
      $\operatorname{LSE}(s_{\mathrm{local}}(q))$, \\
      $\operatorname{LSE}(s_{\mathrm{sink}}(q'))$,
      $\operatorname{LSE}(s_{\mathrm{cpu}}(q'))$,
      $\operatorname{LSE}(s_{\mathrm{local}}(q'))$.
\item $\|O_{\mathrm{sink}}(q)\|_2$, $\|O_{\mathrm{local}}(q)\|_2$, \\
      $\|O_{\mathrm{sink}}(q')\|_2$, $\|O_{\mathrm{cpu}}(q')\|_2$, $\|O_{\mathrm{local}}(q')\|_2$.
\end{itemize}

Practical note (CPU segment). During decoding, $V_{\mathrm{cpu}}$ is resident in host memory; therefore, $\|O_{\mathrm{cpu}}(q)\|_2$ is not used as a feature to avoid expensive host access. Instead, we approximate the scalar $\operatorname{LSE}(s_{\mathrm{cpu}}(q))$ using precomputed moments. Specifically, we approximate
\[
\operatorname{LSE}(s_{\mathrm{cpu}}(q))
\approx \log (L_{\mathrm{cpu}}) + \|q\|_2 \mu_q + \tfrac{1}{2}\|q\|_2^2 \sigma_q^2,
\]
where $\mu_q \approx \frac{\langle q, \operatorname{MEAN}(K_{\mathrm{cpu}})\rangle}{\|q\|_2 \sqrt{D}}$, $\sigma_q^2 \approx \operatorname{VAR}(z(q'))$.

\noindent{\textbf{Query Dynamics Features (3).}}
These features capture temporal consistency between the current decoding query and the anchor query.
\begin{itemize}
\item $\|q\|_2$, $\|q'\|_2$.
\item $\dfrac{\langle q,q'\rangle}{\|q\|_2\,\|q'\|_2}$.
\end{itemize}

\noindent{\textbf{Budget Estimation Features (4).}}
Using $q'$ as the anchor query, we apply the KV budget allocation criterion in Eq.~\ref{eq:min-bgt} under different block-wise selection granularities, i.e., $\mathrm{blk} \in \{16, 32, 64, 128\}$.

\begin{itemize}
\item $bgt^*(16)$, $bgt^*(32)$, $bgt^*(64)$, $bgt^*(128)$.
\end{itemize}

\noindent{\textbf{Cross-head Features (2).}}
To capture cross-head disparity, we use the maximum head output magnitude as a global indicator.
Since the full $\|O_{h'}(q)\|_2$ is not available before computing attention over CPU-resident values, we approximate it using GPU-resident tokens only. Define
\[
O_{h'}(q) \approx \widetilde{O}_{h'}(q) = \operatorname{softmax}\!\Bigl(\frac{q_{h'}K_{\mathrm{gpu},h'}^\top}{\sqrt{D}}\Bigr)\,V_{\mathrm{gpu},h'}.
\]
We then use:
\begin{itemize}
\item $\max_{h'=1}^{H}\|\widetilde{O}_{h'}(q)\|_2$, $\max_{h'=1}^{H}\|\widetilde{O}_{h'}(q')\|_2$.
\end{itemize}

\subsection{Feature Extraction}
\label{app:feature_extraction}

\noindent{\textbf{Offline training.}}
In the offline training stage, we pair each 41-dimensional feature vector with its corresponding label tuple $\{bgt_{h,0}, k_h, s_h\}$ from LongBench V2~\cite{bai2024longbench2}. We standardize each feature dimension using training-set statistics and normalize it accordingly. The same normalization statistics are reused during inference to ensure consistent scaling.

\noindent{\textbf{Online inference.}} 
During the prefill stage, we compute structural features, KV distribution features, and moment statistics based on the anchor query $q'$. All CPU-segment statistics (e.g., $\operatorname{MEAN}(K_{\mathrm{cpu}})$) and $q'$ are cached, thereby avoiding any subsequent access to CPU-resident KV tensors. We further compute $q'$-dependent attention contribution features as well as budget estimation features $\{bgt^*(blk)\}$.


At each decoding step, given the current query $q$, we update query-dependent features such as $\|q\|_2$, cosine similarity with $q'$, and sink/local segment LSE and output norms. The CPU-segment $\operatorname{LSE}(s_{\mathrm{cpu}}(q))$ is computed via the moment-based approximation described above. All extracted features are obtained via CUDA Graph–optimized execution, and are subsequently normalized using pre-computed training statistics before being fed into the predictor for final predictions.
